# Supplementary material for: Latent Space Translation via Inverse Relative Projection
Source: arXiv:2406.15057 source file (2024-06-21)
Supplement: Supplementary file 1 [file 7.supmat.tex]

\begin{figure}[h]
    \centering
    \begin{overpic}[clip,width=1\linewidth]{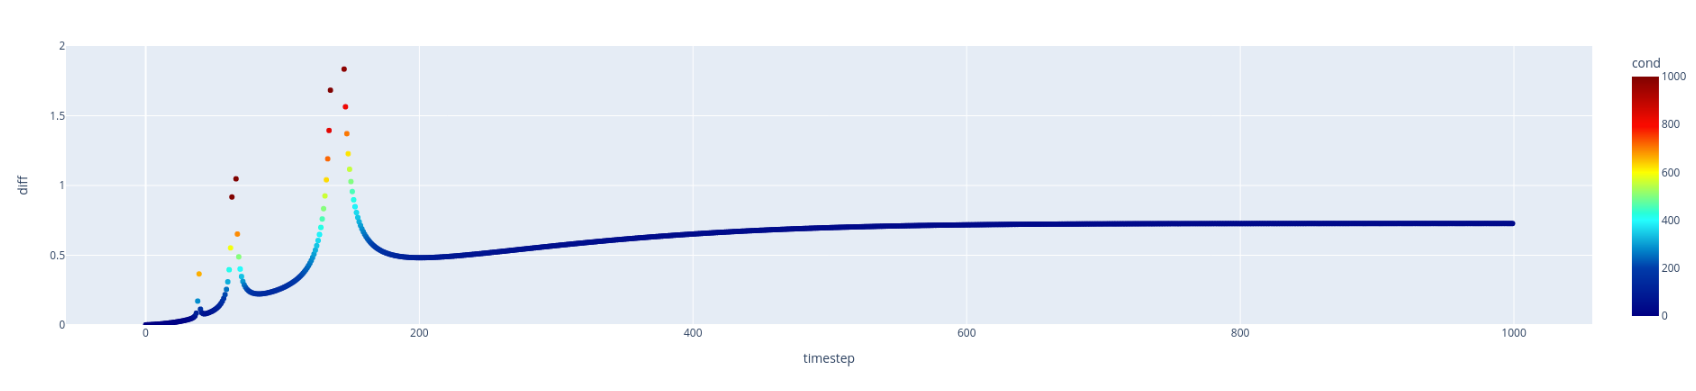}
        %  trim={<left> <lower> <right> <upper>}
        %  \put(horiz, vert)
        %  \put(horiz, vert){\rotatebox{90}{Text}}
        %
    \end{overpic}
  
    \caption{TBA  }
    \label{fig:anchors-diffusion}
\end{figure}

\begin{figure}[h]
    \centering
    \begin{overpic}[clip,width=.5\linewidth]{example-image-a}
        %  trim={<left> <lower> <right> <upper>}
        %  \put(horiz, vert)
        %  \put(horiz, vert){\rotatebox{90}{Text}}
        %
    \end{overpic}
  
    \caption{Something to show that we can reconstruct the absolute spaces starting from a relative one, using only the anchor set. Maybe a formula is better?}
    \label{?}
\end{figure}

\begin{figure}[h]
    \centering
    \begin{overpic}[clip,width=1\linewidth]{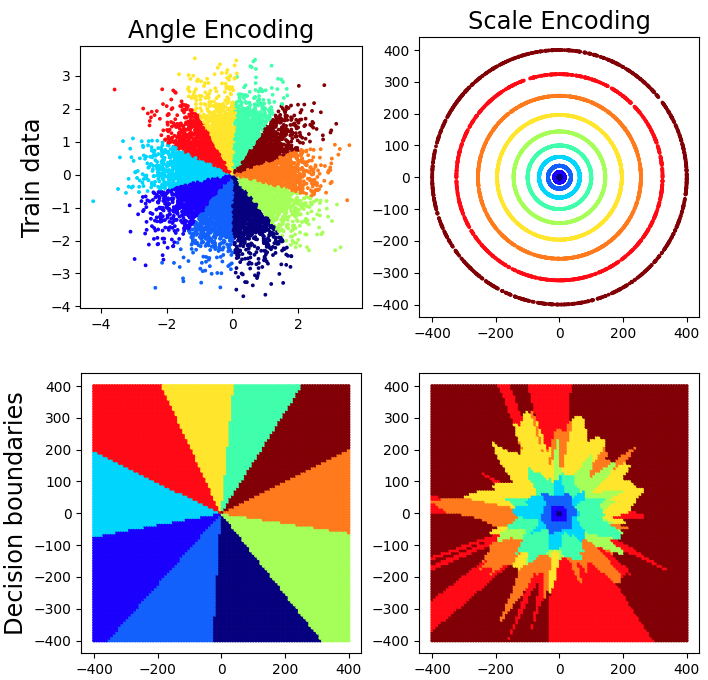}
        %  trim={<left> <lower> <right> <upper>}
        %  \put(horiz, vert)
        %  \put(horiz, vert){\rotatebox{90}{Text}}
        %
    \end{overpic}
  
    \caption{TBA {Luca: Aggiungere una riga con il rescaling per far vedere che uno si rompe l'altro no}}
    \label{fig:scale-invariance-synthetic}
\end{figure}

\paragraph{Word Embeddings scale}
The well-known word embeddings, FastText and Word2Vec, exhibit a scale-invariant behavior. As shown in \Cref{fig:norm-ranges}, there is a clear separation between the FastText and Word2Vec norms and no correlation between the norms of the same words represented in the two spaces. This observation suggests that in this case, there is no semantically relevant information encoded in the norms. These results indicate that the scale of the embedding does not play a significant role in the performance of these word embedding models.

\paragraph{Big models scale-invariance}
We observed that large pre-trained models, such as transformers and resnets, are robust to internal rescaling of the encodings. Although we do not have a clear explanation for this phenomenon, we hypothesize that normalization layers and the linear separability of the information encoded in the angles instead of the norms (as seen in \Cref{fig:norm-ranges}) may play a role.
In \Cref{fig:rescaled-layer-acc}, we demonstrate the invariance a large transformer exhibits when the rescaling injection is applied at different layers: surprisingly, when the rescaling surpasses a certain threshold, the performance difference becomes negligible.
These results further emphasize the robustness of these pre-trained models to the rescaling injection and suggest that the scale of the embedding is not a critical factor in their performance.

\begin{figure}[h]
    \centering
    \begin{overpic}[clip,width=0.48\linewidth]{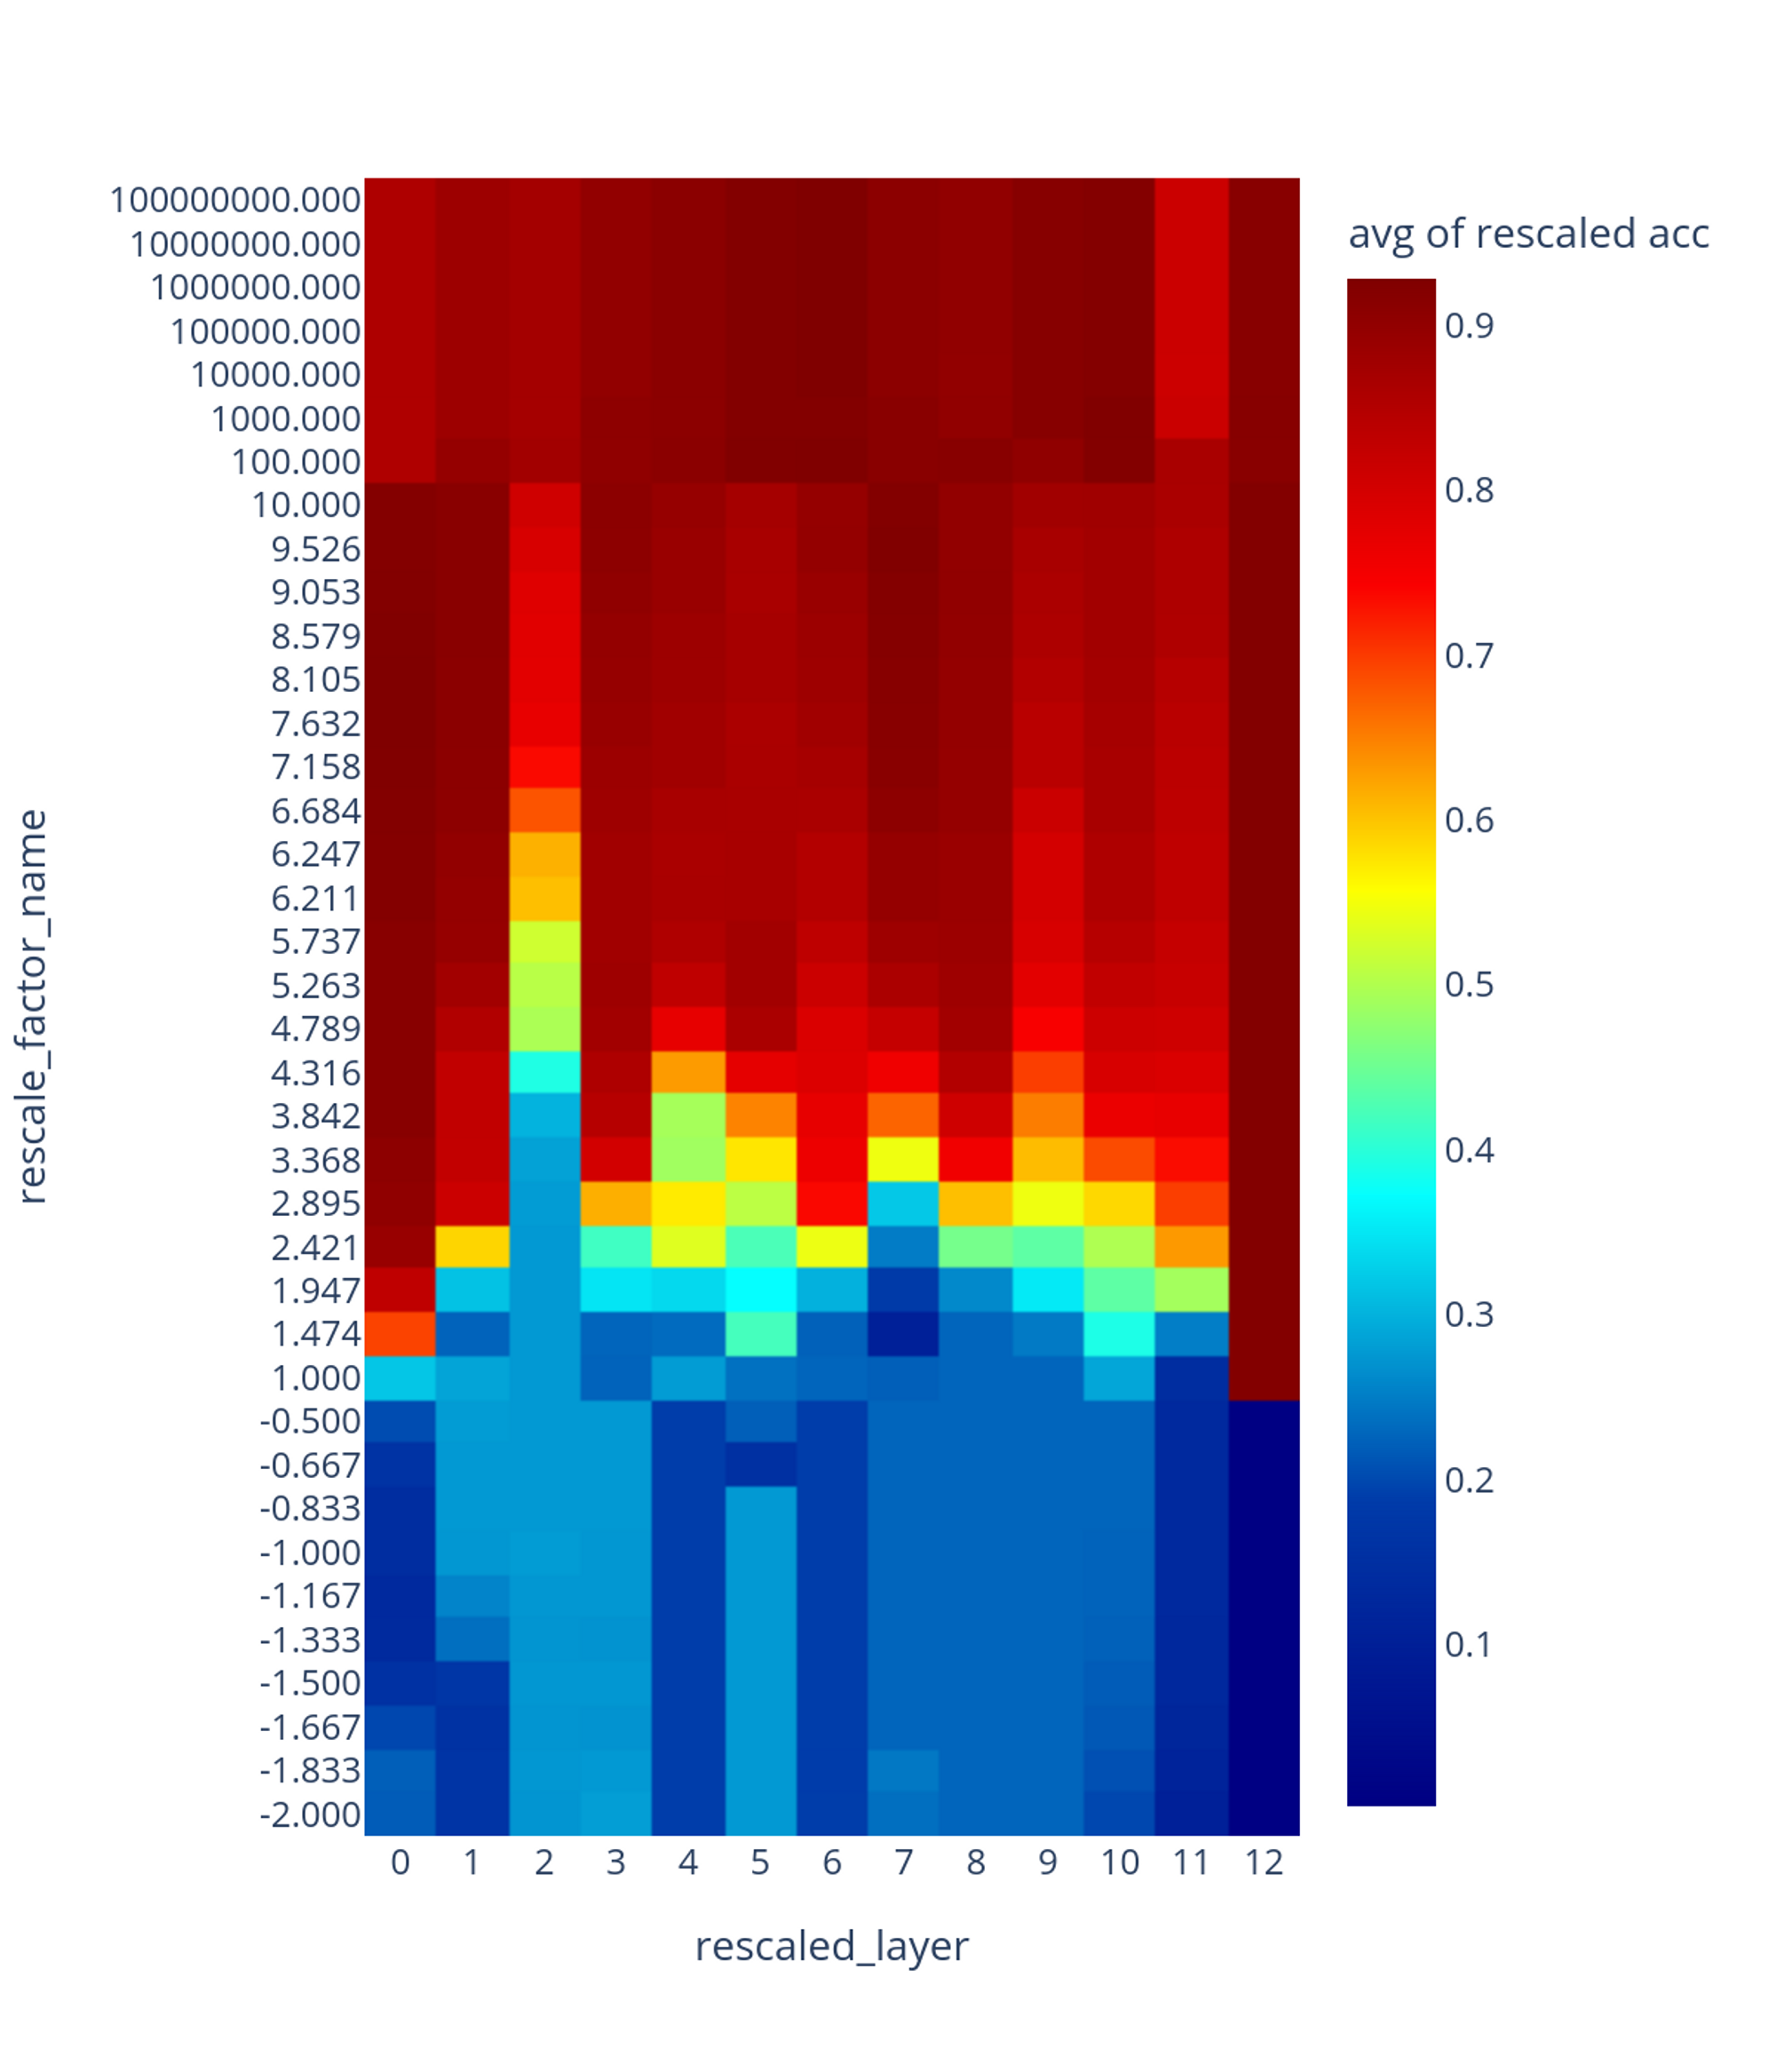}
        %  trim={<left> <lower> <right> <upper>}
        %  \put(horiz, vert)
        %  \put(horiz, vert){\rotatebox{90}{Text}}
        %
    \end{overpic}
    \hfill
    \begin{overpic}[clip,width=0.48\linewidth]{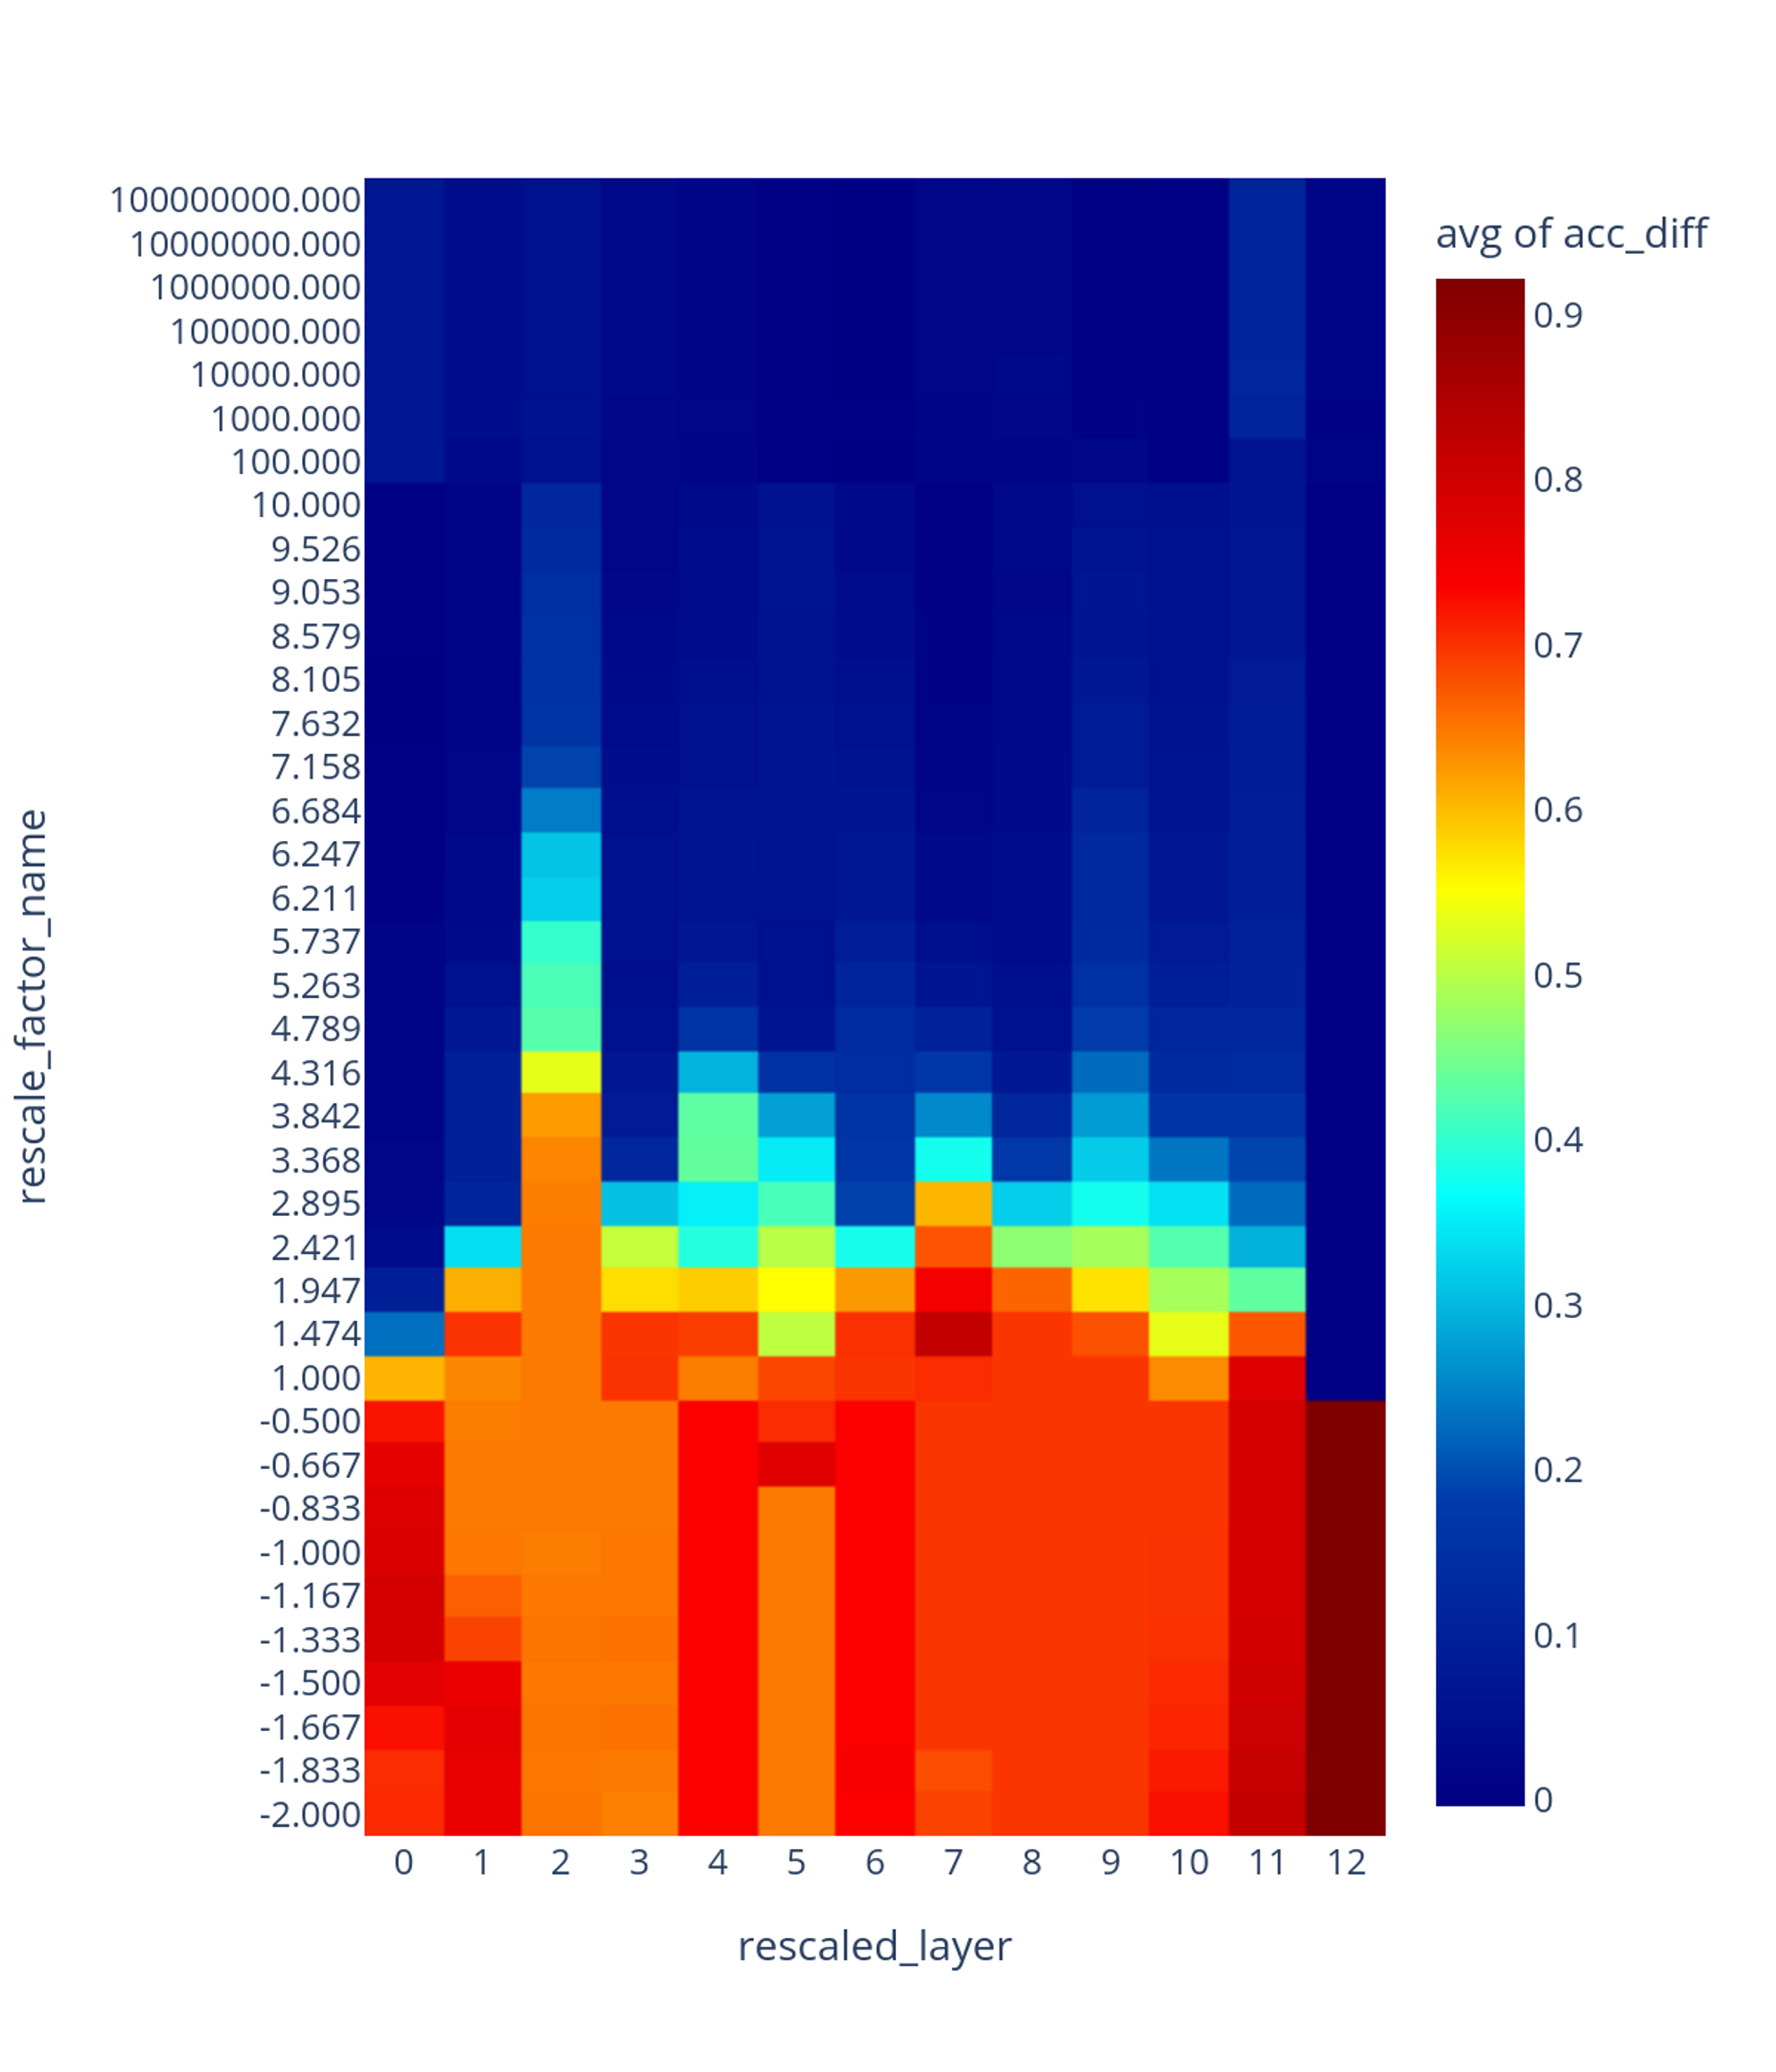}
        %  trim={<left> <lower> <right> <upper>}
        %  \put(horiz, vert)
        %  \put(horiz, vert){\rotatebox{90}{Text}}
        %
    \end{overpic}
    \caption{TBA: \luca{ refactor the images to be horizontal that fit better the template}}
    \label{fig:rescaled-layer-acc}
\end{figure}

\paragraph{Decoder scale-invariance}
We surprisingly observed that even MLPs trained on top of big models learn to be invariant to the rescale injection, as shown in \Cref{fig:decoder-norm-invariance}. We have complete control over the MLPs and surely they should not be invariant to rescaling by construction. 

Overall, these observation provide the foundation that enable the zero-shot stitching between independently pre-trained neural components that we will explore in the next section.

 \begin{figure}[h]
    \centering
    \begin{overpic}[clip,width=1\linewidth]{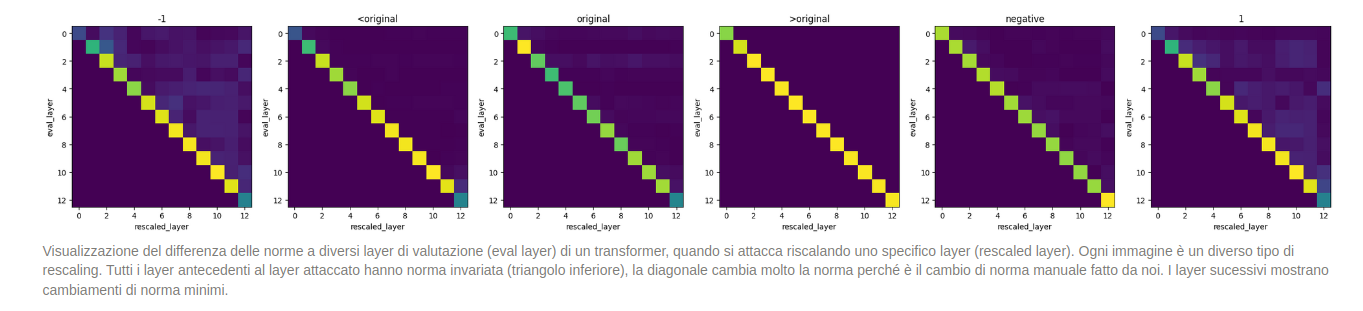}
        %  trim={<left> <lower> <right> <upper>}
        %  \put(horiz, vert)
        %  \put(horiz, vert){\rotatebox{90}{Text}}
        %
    \end{overpic}
  
    \caption{TBA transformer-norm-invariance}
    \label{fig:transformer-norm-invariance}
\end{figure}

\begin{figure}[h]
    \centering
    \begin{overpic}[clip,width=1\linewidth]{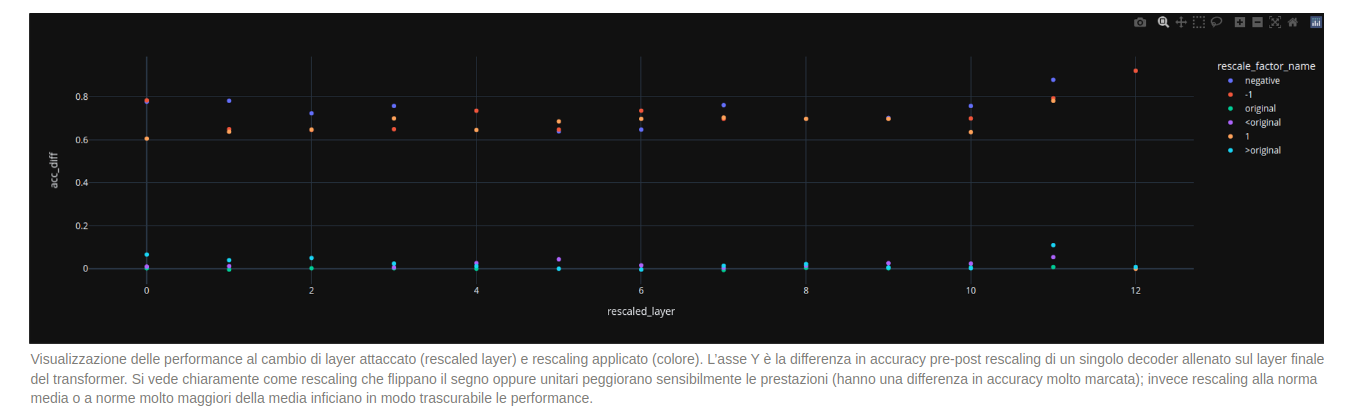}
        %  trim={<left> <lower> <right> <upper>}
        %  \put(horiz, vert)
        %  \put(horiz, vert){\rotatebox{90}{Text}}
        %
    \end{overpic}
  
    \caption{TBA decoder-norm-invariance}
    \label{fig:decoder-norm-invariance}
\end{figure}

\begin{table}
\centering
\caption{TBA}
\label{tab:cross-space-inversion}
\begin{tabular}{llrrr}
\toprule
   &    &  mono similarity &  multi similarity &  rec similarity \\
encoding lang & decoding lang &                  &                   &                 \\
\midrule
\multirow{4}{*}{en} & en &             1.00 &              1.00 &            0.97 \\
   & es &             0.00 &              0.99 &            0.93 \\
   & fr &            -0.02 &              0.99 &            0.70 \\
   & ja &             0.03 &              0.99 &            0.84 \\
\cline{1-5}
\multirow{4}{*}{es} & en &             0.00 &              0.99 &            0.97 \\
   & es &             1.00 &              1.00 &            0.94 \\
   & fr &             0.01 &              0.99 &            0.69 \\
   & ja &             0.00 &              0.99 &            0.84 \\
\cline{1-5}
\multirow{4}{*}{fr} & en &            -0.02 &              0.99 &            0.97 \\
   & es &             0.01 &              0.99 &            0.93 \\
   & fr &             1.00 &              1.00 &            0.70 \\
   & ja &            -0.02 &              0.99 &            0.84 \\
\cline{1-5}
\multirow{4}{*}{ja} & en &             0.03 &              0.99 &            0.97 \\
   & es &             0.00 &              0.99 &            0.93 \\
   & fr &            -0.02 &              0.99 &            0.69 \\
   & ja &             1.00 &              1.00 &            0.85 \\
\bottomrule
\end{tabular}
\end{table}

\begin{table}[h]
\centering
\caption{HuggingFace transformers used in \Cref{?} to for cross-lingual transfer.}
\label{tab:transformers-nlp}
\begin{tabular}{lll}
\toprule
Language & HuggingFace transformers name    & Encoding Dim \\
\midrule
English  & openai/clip-vit-base-patch32     & 768          \\
English  & bert-base-cased                  & 768          \\
English  & roberta-base                     & 768          \\
English  & xlm-roberta-base                 & 768          \\
English  & google/electra-base-discriminator                 & 768          \\
Spanish  & PlanTL-GOB-ES/roberta-base-bne   & 768          \\
French   & ClassCat/roberta-base-french     & 768          \\
Japanese & nlp-waseda/roberta-base-japanese & 768          \\
\bottomrule
\end{tabular}
\end{table}
